# Supplementary material for: Consistency Learning via Decoding Path Augmentation for Transformers in Human Object Interaction Detection
Source: arXiv:2204.04836 source file (2022-04-11)
Supplement: Supplementary file 1 [file supple_asnet.tex]

\begin{table}[!h]
    \centering
    \footnotesize
    % \caption{Ablation.}
    
    \begin{tabular}{l c c   c  c c }
         \toprule
         \multicolumn{1}{c}{} &
         \multicolumn{2}{c}{} &
         \multicolumn{3}{c}{HICO-DET} \\

         \cmidrule(r){4-6}
         Method & 
         epoch &
         $\lambda$&
         $\  $ {Full} $\  $ & 
         {Rare} & 
         {Non-Rare   }
         \\
         \midrule
         \midrule
         
        %  \rowcolor{Gray} 
        %  \multicolumn{6}{l}{ \text{Single-decoder HOI transformer}}   
        %  \\ \midrule
        
        %  \rowcolor{Gray}\multicolumn{6}{l}{ \text{Two-decoder HOI transformer}}   \\ \midrule
         
         AS-Net&90&-&28.87& 24.25&30.25\\
         AS-Net + ours&90&0.5&\textbf{29.13}&\textbf{25.18} &\textbf{30.31}  \\
         \bottomrule
    \end{tabular}
    \caption{\textbf{Comparison of our training strategy with AS-Net on HICO-DET}. 
    }
    \label{table:supple_asnet}
    
\end{table}
