# Supplementary material for: Consistency Learning via Decoding Path Augmentation for Transformers in Human Object Interaction Detection
Source: arXiv:2204.04836 source file (2022-04-11)
Supplement: Supplementary file 2 [file supple_coef_hotr.tex]

\begin{table}[!h]
    \centering
    \footnotesize
    % \caption{Ablation.}
    
    \begin{tabular}{l  c c  c }
         \toprule

         Dataset 
         & epoch
         & $\lambda$ 
         & $t_\text{max}$
         \\
         \midrule
         \midrule
         
        %  \rowcolor{Gray} 
        %  \multicolumn{6}{l}{ \text{Single-decoder HOI transformer}}   
        %  \\ \midrule
        
        V-COCO 
        & 90
        & 1
        & 30\\
       
         \midrule
         
        %  \rowcolor{Gray}\multicolumn{6}{l}{ \text{Two-decoder HOI transformer}}   \\ \midrule
         
         HICO-DET
        & 50
        & 0.2
        & 20\\
         \bottomrule
    \end{tabular}
    %\caption{\textbf{Hyperparameters for the weight scheduler for HOTR}}
    % \caption{\textbf{Weight scheduler for total CPC loss for HOTR}}
    \caption{\textbf{Weight scheduler settings for HOTR}}
    % \caption{\textbf{Total CPC loss coefficient for HOTR}}
    \label{table:hotr-coef}
    
\end{table}
