# Supplementary material for: Consistency Learning via Decoding Path Augmentation for Transformers in Human Object Interaction Detection
Source: arXiv:2204.04836 source file (2022-04-11)
Supplement: Supplementary file 4 [file supple_hoit.tex]

% \begin{table}[!h]
%     \centering
%     \footnotesize
%     % \caption{Ablation.}
    
%     \begin{tabular}{l c c   c   }
%          \toprule
%          \multicolumn{1}{c}{} &
%          \multicolumn{2}{c}{} &
%          \multicolumn{3}{c}{V-COCO} \\

%          \cmidrule(r){4}
%          Method & 
%          epoch &
%          $\lambda$&
%          $\scone $ & 
%          \\
%          \midrule
%          \midrule
         
%         %  \rowcolor{Gray} 
%         %  \multicolumn{6}{l}{ \text{Single-decoder HOI transformer}}   
%         %  \\ \midrule
        
%         %  \rowcolor{Gray}\multicolumn{6}{l}{ \text{Two-decoder HOI transformer}}   \\ \midrule
         
%         HoiT & 150 & & 48.75* &  \\
%         HoiT + ours & 150 & 0.2 &49.34& \\
%          \bottomrule
%     \end{tabular}
%     \caption{\textbf{Comparison of our training strategy with HoiT on V-COCO and HICO-DET}. 
%     * signifies our results reproduced with the official implementation codes of ~\cite{HOITR}.}
    
%     \label{table:supple_hoit}
    
% \end{table}

\begin{table}[!h]
    \centering
    \footnotesize
    % \caption{Ablation.}
    
    \begin{tabular}{l c c   l}
         \toprule
         \multicolumn{1}{c}{} &
        %  \multicolumn{2}{c}{} &
         \multicolumn{3}{c}{V-COCO} \\
         \cmidrule(l){2-4}
         Method & 
         epoch &
         $\lambda$&
         \scone 
         \\
         \midrule
         \midrule
         
        %  \rowcolor{Gray} 
        %  \multicolumn{6}{l}{ \text{Single-decoder HOI transformer}}   
        %  \\ \midrule
        
        %  \rowcolor{Gray}\multicolumn{6}{l}{ \text{Two-decoder HOI transformer}}   \\ \midrule
         
          HoiT&150&-&48.75*\\
         HoiT + ours&150&0.2&\textbf{49.34} \\
         \bottomrule
    \end{tabular}
    \caption{\textbf{Comparison of our training strategy with HoiT on V-COCO}. * signifies our results reproduced with the official implementation codes of~\cite{HOITR}. 
    }
    \label{table:supple_hoit}
    
\end{table}
